# Supplementary material for: Discrete Sequential Prediction of Continuous Actions for Deep RL
Source: arXiv:1705.05035 source file (2019-06-08)
Supplement: Supplementary file 1 [file appendix_c.tex]

%%% NOT USED

\section{Constant value Q surfaces}
\begin{figure}
 \centering
  \includegraphics[width=\linewidth]{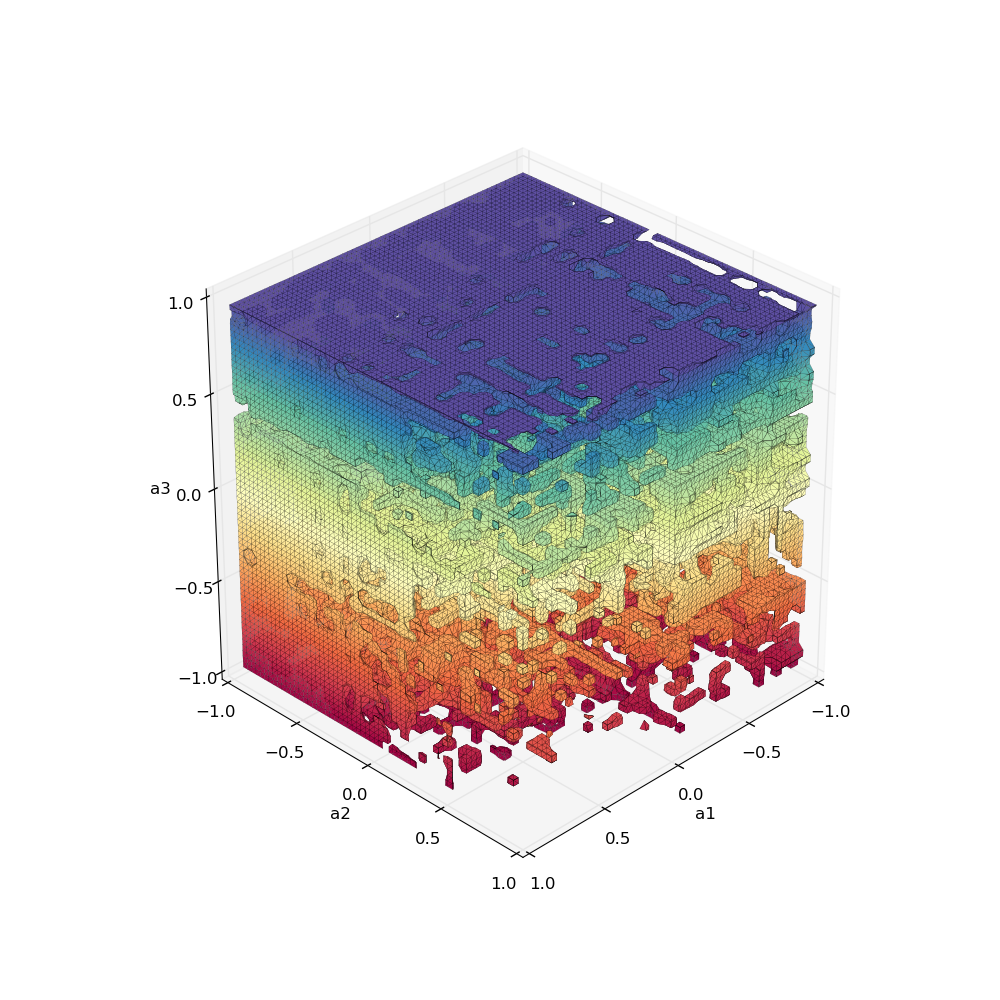}
  \caption{constant value q surface for $Q^D$ on a Max SDQN model trained on hopper}
\end{figure}

\begin{figure}
 \centering
  \includegraphics[width=\linewidth]{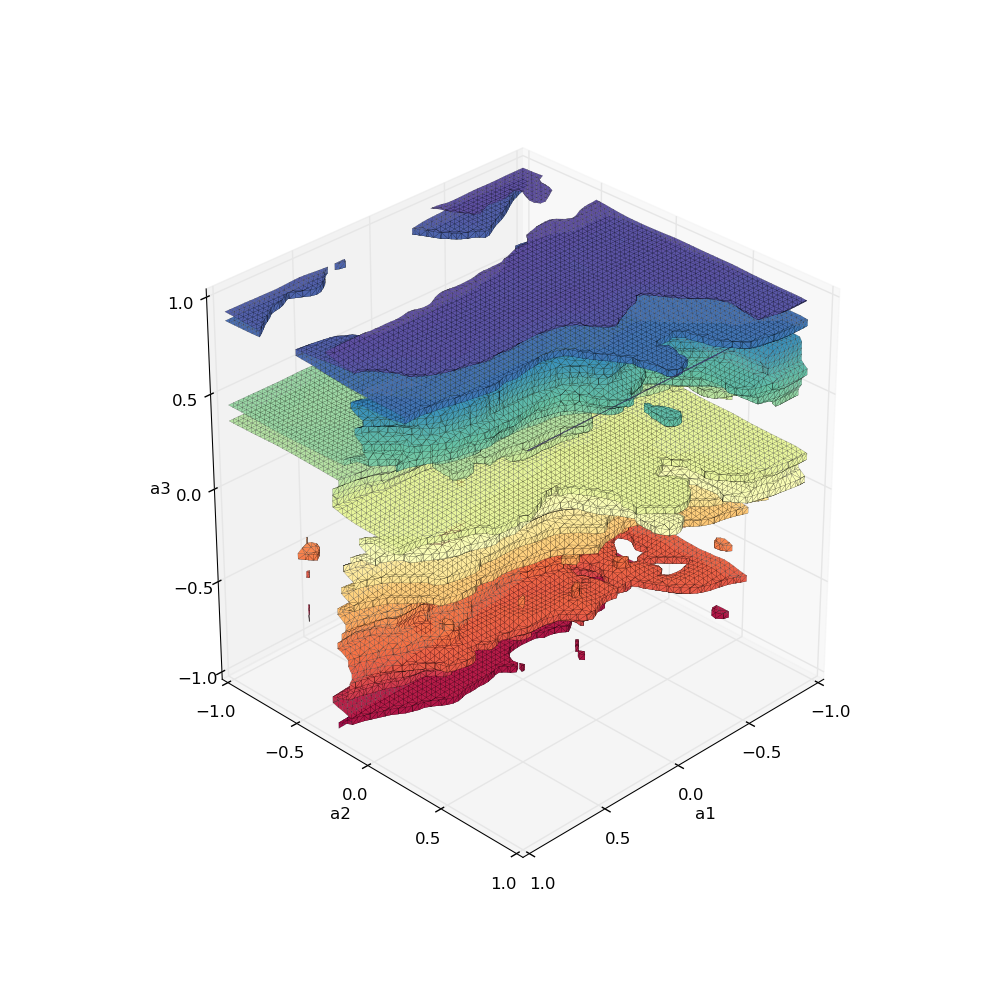}
  \caption{constant value q surface for $Q^D$ on a Max SDQN model trained on hopper}
\end{figure}
